# Supplementary material for: Measurement of $CP$ observables in $B^{\pm} \to D K^{\pm}$ and $B^{\pm} \to D \pi^{\pm}$ with $D \to K_{\rm{S}}^0 K^\pm \pi^\mp$ decays
Source: arXiv:2002.08858 source file (2020-06-11)
Supplement: Supplementary file 3 [file supplementary.tex]

\section{Inclusion of supplementary material}
\label{sec:Supplementary}

Three types of supplementary material should be distinguished:
\begin{itemize}
\item{A regular appendix: lengthy equations or long tables are sometimes
better put in an appendix in order not to interrupt the main flow of a paper.
Appendices will appear in the final paper, on arXiv
and on the CDS record and should be considered integral
part of a paper, and are thus to be reviewed like the rest of the paper.
An example of an LHCb paper with an appendix is Ref.~\cite{LHCb-PAPER-2013-070}.
}
\item{Supplementary material for CDS: plots or tables that 
would make the paper exceed the page limit or are
not appropriate to include in the paper itself,
but are desirable to be shown in public
should be added to the paper drafts in an appendix, and
removed from the paper before submitting to arXiv or the journal.
See Appendix~\ref{sec:Supplementary-App} for further instructions.
Examples are: comparison plots of the new result with older results,
plots that illustrate cross-checks.
An example of an LHCb paper with supplementary material for CDS 
is Ref.~\cite{LHCb-PAPER-2013-035}.
Supplementary material for CDS cannot be referenced in the paper.
Supplementary material should be included in the draft paper to be
reviewed by the collaboration.
}
\item{Supplementary material for the paper. This is usually called ``supplemental material'', which distinguishes it from supplementary material for CDS only. Most journals allow
to submit files along with the paper that will not be part of the
text of the article, but will be stored on the journal server.
Examples are plain text files with numerical data corresponding to the plots
in the paper. 
The supplemental material should be cited in the paper by including a reference
which should say ``See supplemental material at [link] for [give brief description of material].''
The journal will insert a specific link for [link]. The arXiv version will usually include the supplemental material as part of the paper and so should not contain the words ``at [link]''.
Supplemental material should be included in the draft paper to be
reviewed by the collaboration.
An example of an LHCb paper with supplemental material 
is Ref.~\cite{LHCb-PAPER-2015-029}
}
\end{itemize}
